# Supplementary material for: Almost local generation of EPR entanglement in non-equilibrium
Source: arXiv:1305.6566 ancillary file (2013-07-26)
Supplement: Supplementary file 1 [file supplement_RSchmidt.pdf]

# Quasi-local generation of EPR entanglement in non-equilibrium: Supplemental Material

Rebecca Schmidt,* Jürgen T. Stockburger, and Joachim Ankerhold

*Institut für Theoretische Physik, Universität Ulm,*

*Albert Einstein-Allee 11, 89069 Ulm, Germany*

(Dated: May 28, 2013)

## Abstract

In this supplemental material to our article 'Quasi-local generation of EPR entanglement in non-equilibrium' [ ref: article] the dynamics of the parametric quantum oscillator is reviewed with emphasis on the time evolution of the covariance matrix. We also outline some technical details of the optimization algorithm we use.

* rebecca.schmidt@uni-ulm.de

## I. PARAMETRIC QUANTUM OSCILLATOR

### A. Classical dynamics

The classical equation of motion for a damped harmonic oscillator parametrically driven by a control field $u(t)$ reads in dimensionless units as used in the main text

$$\ddot{q}(t) + \eta \dot{q}(t) + \omega(t)^2 q(t) = 0 \tag{1}$$

where $\omega(t)^2 = 1 + u(t)$. In the sequel, friction is considered as weak $\eta \ll 1$ and about the control signal we only assume that it is sufficiently smooth and bounded from below such that $\omega(t)^2 \geq 0$. Then, solutions to (1) can be written in the form $q(t) = \mathrm{e}^{-\eta t/2}\, Q(t)$ where

$$\ddot{Q}(t) + \tilde{\omega}(t)^2 Q(t) = 0 \tag{2}$$

with $\tilde{\omega}(t)^2 = \omega(t)^2 - \eta^2/4 \approx \omega(t)^2$ in the weak friction limit. Relevant observables can then be expressed in terms of the independent solutions $\phi_k(t), k = 1, 2$ of (2) with initial conditions $\phi_1 = 0, \dot{\phi}_1(0) = 1$ and $\phi_2(0) = 1, \dot{\phi}_2(0) = 0$. According to Abel's identity [1] the corresponding Wronskian then obeys

$$\phi_2(t)\dot{\phi}_1(t) - \phi_1(t)\dot{\phi}_2(t) = 1\,. \tag{3}$$

Further properties about the $\phi_i$ are known only in case of a purely periodic drive, e.g. $u(t) = a\cos(2\omega_0 t)$ (see [2]). Even though typical optimal control signals are *not* of this

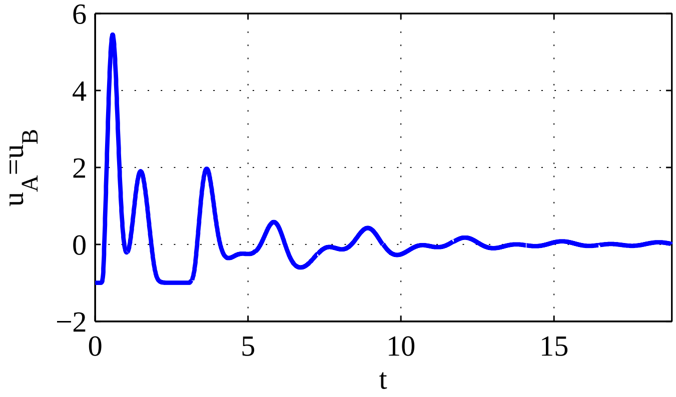


FIG. 1. Optimized control signal for symmetric two-site control for the parameters in Fig. 2 of the main text.

simple form (cf. Fig. 1), it is instructive to recall some results: solutions are of the form $\phi_1(t) = [F_\nu(t) - F_\nu(-t)]/[2\dot{F}_\nu(0)]$ and $\phi_2(t) = [F_\nu(t) + F_\nu(-t)]/[2F_\nu(0)]$ where the Mathieu function $F_\nu(t) = \exp(i\nu t)\, p(t)$ contains the Floquet exponent $\nu$ and a periodic function $p(t) = p(t + \pi/\omega_0)$; orbits of (1) are found to be unstable if $|\mathrm{Im}\{\nu\}| > \eta/2$.

### B. Parametrization of Gaussian quantum states

A Gaussian state is fully characterized the expectation values of conjugate variables $q$ and $p$, and by its covariance matrix $\sigma_{xy} = \frac{1}{2}\langle xy+yx\rangle - \langle x\rangle\langle y\rangle$, $x, y \in \{q, p\}$. The matrix elements of $\sigma$ themselves are suitable as dynamical variables (see below), however, the parametrization

$$\sigma_{qq} = a^2\,(\cosh 2r + \cos 2\varphi \sinh 2r) \tag{4}$$

$$\sigma_{qp} = -a^2 \sin 2\varphi \sinh 2r \tag{5}$$

$$\sigma_{pp} = a^2\,(\cosh 2r - \cos 2\varphi \sinh 2r) \tag{6}$$

through a squeezing parameter $r$, a squeezing angle $\varphi$, and a width parameter $a$ with $\sigma_{qq}\sigma_{pp} - \sigma_{qp}^2 = a^4$ is often more suitable to discuss qualitative properties of a quantum state [3]. Alternatively, the width parameter $a$ can be replaced by an effective temperature parameter through

$$a^2 = \frac{1}{2}\coth\frac{\beta}{2}. \tag{7}$$

For the case of symmetric driving discussed in the main paper, the two-mode covariance matrix factorizes when transformed to normal modes. It is therefore determined by the parameter set $r_\pm$, $\varphi_\pm$, $a_\pm$. Using this parameter set, and reverting to local modes, the quantity $\det\gamma$ (see main paper), takes the form

$$\det\gamma = \frac{1}{2}\left[a_+^4 + a_-^4 - 2a_+^2 a_-^2(\cosh 2r_- \cosh 2r_+ - \cos(2\varphi_- - \varphi_+)\sinh 2r_- \sinh 2r_+)\right] \tag{8}$$

The condition $\det\gamma < 0$ translates thus into

$$\cosh 2r_- \cosh 2r_+ - \cos(2\varphi_- - 2\varphi+)\sinh 2r_- \sinh 2r_+ > \frac{1}{2}\left(\frac{a_+^2}{a_-^2} + \frac{a_-^2}{a_+^2}\right). \tag{9}$$

### C. Quantum dynamics

In the quantum regime, the variances $\sigma_{xy} = \frac{1}{2}\langle xy + yx\rangle - \langle x\rangle\langle y\rangle$, $x, y \in \{q, p\}$ of the conjugate operators $q, p$ are the interesting quantities. In the undamped case ($\eta = 0$) they

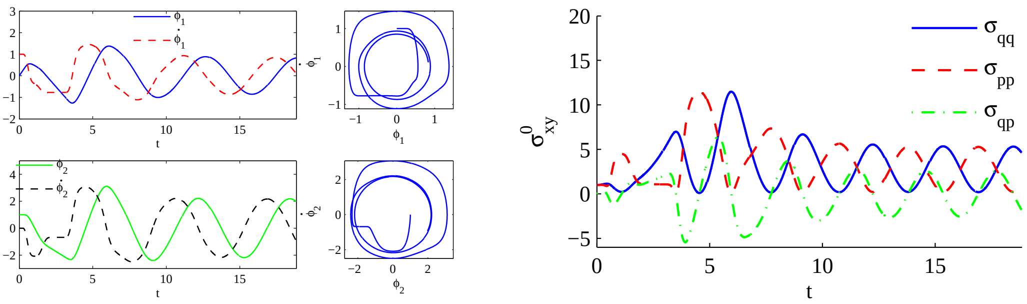


FIG. 2. Left: Time evolution of functions $\phi_1(t)$ and $\phi_2(t)$ (solid) and their respective derivatives (dashed) for the optimal control signal $u(t)$ obtained for the two-site controlled quantum dynamics with parameters as in Fig. 2 of the main text. Middle: Corresponding phase space orbits. Right: Time evolution of the quadrature variances of a non-dissipative parametric quantum oscillator driven by the same optimal control signal $u(t)$.

obey the following set of equations

$$\dot{\sigma}_{qq}^{(0)} = 2\sigma_{qp}^{(0)} \ , \ \dot{\sigma}_{pp}^{(0)} = -2\omega(t)^2\sigma_{qp}^{(0)} \ , \ \dot{\sigma}_{qp}^{(0)} = \sigma_{pp}^{(0)} - \omega(t)^2\sigma_{qq}^{(0)} \, . \tag{10}$$

For a ground state as initial state one has $\sigma_{qq}(0) = \sigma_{pp} = 1, \sigma_{qp} = 0$ and finds

$$\sigma_{qq}^{(0)}(t) = \phi_1(t)^2 + \phi_2(t)^2 \ , \ \sigma_{pp}^{(0)}(t) = \dot{\phi}_1(t)^2 + \dot{\phi}_2(t)^2 \ , \ \sigma_{qp}^{(0)}(t) = \phi_1(t)\dot{\phi}_1(t) + \phi_2(t)\dot{\phi}_2(t) \, . \tag{11}$$

The calculation for a dissipative system is much more cumbersome. It can conveniently be performed using techniques from [4] in terms of the path integral representation of the reduced density operator of the system. For the variances one then obtains $\sigma_{xy}(t) = \sigma_{xy,0}(t) + \sigma_{xy,\beta}(t)$, where the first transient part depends on the initial state but is independent of temperature while the second non-decaying part depends on temperature only. Approximately, in the weak friction limit one has $\sigma_{xy,0}(t) \sim \exp(-\eta t)\sigma_{xy}^{(0)}(t)$. Further, the non-decaying parts of the variances take the form [4] $\sigma_{qq,\beta}(t) = a_{qq}(t)$ so that $\sigma_{pp,\beta}(t) = \ddot{a}_{qq}(t)$, and $\sigma_{qp,\beta}(t) = \dot{a}_{qq}(t)$ where

$$a_{qq}(t) = \int_0^t ds \int_0^s du \, \varphi(t,s) \, K(s-u) \, \varphi(t,u) \, \mathrm{e}^{-\eta[t-(s+u)/2]} \, . \tag{12}$$

This includes the real part of the reservoir force-force correlation

$$K(s) = \int_0^\infty \frac{d\omega}{\pi} \, J(\omega) \, \coth(\omega\hbar\beta/2) \, \cos(\omega s) \tag{13}$$

and a function $\varphi(t,s) = [\phi_1(t)\phi_2(s) - \phi_1(s)\phi_2(t)]$ which obeys the classical equation (2) with boundary conditions $\varphi(t,0) = \phi_1(t)$, $\varphi(t,t) = 0$. Further, $d\varphi(t,s)/ds|_{s=t} = -1$ according to (3).

The momentum variance reads $\sigma_{pp,\beta}(t) = a_{pp}(t) + 2a_{qq}(t)\dot{\phi}_1(t)^2/\phi_1(t)^2 + a_{qp}(t)\dot{\phi}_1(t)/\phi_1(t)$ with

$$a_{pp}(t) = \int_0^t ds \int_0^s du \frac{\phi_1(s)}{\phi_1(t)}\, K(s-u)\, \frac{\phi_1(u)}{\phi_1(t)}\, \mathrm{e}^{-\eta[t-(s+u)/2]} \tag{14}$$

and

$$a_{qp}(t) = \int_0^t ds \int_0^s du \frac{\phi_1(s)}{\phi_1(t)}\, K(s-u)\, \varphi(t,u)\, \mathrm{e}^{-\eta[t-(s+u)/2]}\,. \tag{15}$$

For the mixed variance one finds $\sigma_{qp,\beta}(t) = a_{qq}(t)\dot{\phi}_1(t)/\phi_1(t) + a_{qp}(t)$.

In case of a vanishing drive, this reduces with the known equilibrium variances of the dissipative quantum oscillator. For weak to moderate friction, $J(\omega) = \omega\eta\omega_c^2/(\omega^2 + \omega_c^2)^2$ with a large cut-off $\omega_c$, these differ by slight shifts [5] from the values predicted in the canonical ensemble. The position correlations $\sigma_{qq}$ are somewhat smaller (quantum Zeno effect), and the momentum correlations $\sigma_{pp}$ are increased by a correction $\propto \ln\omega_c$. The equilibrium squeezing parameter $r_\beta$ is thus slightly negative. In the high temperature limit or for very weak friction, all parameters revert to their standard equilibrium values, which are characterized by $r_\beta = 0$, $\varphi_\beta = 0$, and width $a$ related to the physical reservoir temperature by Eq. (7).

This can also be verified in case of finite driving. We first mention that the bath kernel takes for very low temperatures the form $K(s) \sim \eta/s^2, s > 1/\omega_c$ and in the high temperature regime becomes local in time, i.e. $K(s) \sim (\eta/\beta)\,\delta(s)$. Further, for optimized control over an interval $[0, t_f]$ with $t_f$ covering at least a few periods of the bare oscillator, signals $u(t)$ typically consist of an initial segment (about at most two periods of the bare oscillator) with large amplitudes and a second segment with low amplitudes and quasi-periodic behavior, see Fig. 1. Correspondingly, the functions $\phi_1(s), \phi_2(s)$ show an oscillatory behavior similiar to the non-driven case for times $s > \tau$ with $t_f \gg \tau$ as displayed in Fig. 2. This in turn splits the range of the time integration in (12) in a short time domain ($s < \tau$) and a range where the damping dependent exponential dictates the decay. Typically, the contribution of the latter range dominates so that one can write $a_{qq}(t_f) = \langle q^2\rangle_\beta + \epsilon_q(t_f)$ with a smaller time-varying part $\epsilon(t_f)$ of order $\eta\mathrm{e}^{-\eta t_f}\phi_1(t)^2$. A similar analysis shows that $a_{pp}$ in leading order approaches, i.e., $a_{pp}(t_f) = \langle p^2\rangle_\beta + \epsilon_p(t_f)$, while the mixed variances remain smaller

than of order 1. Neglecting these small thermal and dynamical corrections, one may insert the thermal-state parameters $r_+ = 0$, $\phi_+ = 0$, and $a_+ = 1/2 \coth(\beta/2)$ into (9). Observing that the antisymmetric mode is a pure state ($a_- = 1/2$), Eq. (9) then reduces to

$$\cosh 2r_- > \coth \beta, \tag{16}$$

which is Eq. (8) of the main text. This indicates that sufficiently strong squeezing can cancel the destructive effect of thermal fluctuations. However, in any experimental setting there is a highest attainable squeezing parameter $r_-$. Eq. (16) then defines an upper limit for the temperature range that allows entanglement generation.

## II. OPTIMIZATION ALGORITHM FOR ENTANGLEMENT CREATION IN OPEN BIPARTITE GAUSSIAN SYSTEMS

The optimization algorithm used in the main text is an extended version of what has been developed for open quantum dynamics in [6], including the respective supplemental material. In the present case, the Hamiltonian Eqs. (1-3) in the main text

$$\begin{aligned} H = &\sum_{j=A,B} \frac{p_j^2}{2M} + \frac{M\Omega^2}{2} q_j^2 + \frac{u_j(t)}{2} q_j^2 \\ &+(q_A + q_B) \sum_k c_k x_k + (q_A + q_B)^2 \sum_k \frac{c_k^2}{2m_k\omega_k^2} + \sum_k \frac{p_k^2}{2m_k} + \frac{m_k\omega_k^2}{2} x_k^2 \end{aligned} \tag{17}$$

gives rise to the following stochastic Liouville-von Neumann equation for a single noise realization $\xi$:

$$\begin{aligned} \dot{\rho}_{AB,\xi} = &-\frac{\mathrm{i}}{\hbar}[H_A \otimes \mathbf{1}_B, \rho_{AB,\xi}] - \frac{\mathrm{i}}{\hbar}[\mathbf{1}_A \otimes H_B, \rho_{AB,\xi}] + \frac{\mathrm{i}}{\hbar}\xi(t)[q_A + q_B, \rho_{AB,\xi}] \\ &-\frac{\mathrm{i}}{\hbar}\frac{\eta}{2}[q_A + q_B, \{p_A + p_B, \rho_{AB,\xi}\}] \,. \end{aligned} \tag{18}$$

Here, $\rho_{AB,\xi}$ denotes the density operator for one stochastic realization with the *physical* reduced density operator $\rho_{AB}$ obtained after averaging over sufficiently many realizations, i.e., $\rho_{AB} = \mathbb{E}\left[\rho_{AB,\xi}\right]$. The statistics of the noise variable $\xi(t)$ is governed by the quantum correlation function of the environmental fluctuations [7]. From (18) corresponding equations of motions for the first and second cumulants in position and in momentum are easily derived. As shown in the main text (Eq. (6)), the for the optimal control procedure the objective is to maximize the entanglement. Variation of the influence functional

$$F[u_A(t), u_B(t); \sigma(t)] = E_{\mathcal{N}}(\sigma(t_f)) \tag{19}$$

with respect to the control fields and to the state and under the constraint that the equations of motion derived from (18) are to be obeyed, provides us with:

- a set of stochastic equations of motion for the cumulants of the co-state $\Lambda$ with an end time boundary condition (backward propagation)
- an update formula for the control signals.

This system of equations (forward propagation, backward propagation and control update) has to be solved consistently and iteratively. For further details we refer to the supplemental material of [6].

Practically, maximizing the logarithmic negativity $E_{\mathcal{N}} = \max\{0, -\ln(\tilde{\nu}_-)\}$ and thus searching iteratively for solutions with arguments in the log-function decreasing towards zero, poses a numerical problem. Namely, for arguments sufficiently close to zero, the optimization procedure becomes extremely sensitive to the noise averaging. It turns out that for the system in question (two identical oscillators, coupled to a common reservoir) minimizing $\det \gamma$ leads as well to the optimization goal but without numerical instabilities.

---


[1] W. E. Boyce and R. C. DiPrima. *Elementary Differential Equations and Boundary Value Problems.* Wiley, 1986.

[2] N. W. McLachlan. *Theory and Application of Mathieu Functions.* Dover, 1964.

[3] C. Weedbrook, S. Pirandola, R. García-Patrón, N. J. Cerf, T. C. Ralph, J. H. Shapiro, and S. Lloyd. *Rev. Mod. Phys.*, 84:621, 2012.

[4] C. Zerbe and P. Hänggi. *Phys. Rev. E*, 52:1533, 1995.

[5] U. Weiss. *Quantum Dissipative Systems.* World Scientific, 2008.

[6] R. Schmidt, A. Negretti, J. Ankerhold, T. Calarco, and J. T. Stockburger. *Phys. Rev. Lett.*, 107:130404, 2011.

[7] J. T. Stockburger and H. Grabert. *Phys. Rev. Lett.*, 88:170407, 2002.
